# Supplementary material for: Instructed to Bias: Instruction-Tuned Language Models Exhibit Emergent Cognitive Bias
Source: arXiv:2308.00225 source file (2024-03-31)
Supplement: Supplementary file 1 [file 12_appendix.tex]

\clearpage
\appendix

\section{Data Generation}
\label{sec:appendix_data_generation}
% \gabis{Also, I think we should have a central place for examples of the different biases, e.g., in a nice table which can act as reference for readers throughout the paper. Then the text here can interact with the table: ``For the decoy bias, we see in Table ...''}

% \gabis{I think the text here abuses the verb ``create'' here. Maybe before starting to describe each bias, describe this ``creation'' process? Are there any common elements in writing the examples to all biases? }
% \itay{I rephrased every 'create' in here to a more suitable word in each case (not sure if that is what you meant).
% I also added a common element, but most of the description is specific for each bias.}

\input{Sections/Tables/data_numbers}

To thoroughly examine the models and mitigate potential confounders we carefully design a range of prompts to assess the models' susceptibility to the three biases.
We generate an extensive collection of \biaseddataset{} and control samples, encompassing various options' values, textual templates, and permutations of option order.

By employing this approach, we aim to introduce substantial variability among the samples while ensuring independence from the original papers' examples, thus minimizing the risk of data contamination.
We elaborate on the data generation process of each one of the biases.
A table representing the total number of samples in each bias is in Table \ref{appendix:tab:data_numbers}

\subsection{Decoy Effect Data}
\label{subsec:data_gen_decoy}
To generate the data for the decoy effect, we follow \cite{huber1982adding} and compose a set of textual prompts, each posing a selection from four different product categories: cars, phones, frying pans, and real estate properties.
Depending if the sample is from the control or from the \biaseddataset{} dataset, each example involved either two or three product alternatives, each with two attributes - product price and quality rating.

In each conditions, we compared two conditions:
% \nir{`setting' sounds like something you make comparisions within -- not accross.}
% \nir{as i said, i would save the word `bias' for the general effect and measurement; consider calling this `control' and `treatment' instead}
\begin{enumerate}
    \item \textbf{Control -- Two Options} Two options are presented: the \textit{Target Option} and the \textit{Competitor Option}.
    \item \textbf{\Biaseddataset{} -- Third Decoy Option} Three options are presented. In addition to \textit{Target Option} and \textit{Competitor Option}, we added the \textit{Decoy Option}.
    % \item \textbf{False Decoy} Three options are presented. \textit{Target Option} and \textit{Competitor Option},  and we add a third \textit{Decoy Option} which is deliberately chosen \textit{not} to be a decoy option according to the definition to act as a control.
\end{enumerate}

We chose price values according to the actual price ranges from web consumer stores or by prompting the model for a reasonable price range.
We chose low-end and high-end products as our two options in the control condition.

To create the decoy option, we follow \citep{huber1982adding} and create four possible decoys according to the target option, each is worse than the target in the price dimension (more expensive, same quality), or the quality dimension (less quality, same price), or a combination of both.

We constructed variations with different price and quality gaps between the options, five different textual templates, and permutations between the location of each option.

\subsection{Certainty Effect Data}
Similarly to the decoy effect, we follow the original work by \citet{kahneman1979prospect} to generate our data.
In both conditions,  two options for getting prize money with different probabilities are presented. One option is with a lower excepted utility than the other (\textit{Target}) while the other option with a higher excepted utility (\textit{Higher Excepted Value}).

% \nir{could we rewrite this to emphasize that both conditions are the same expect that in the treatment condition `high probability' is actually 1?}
\begin{enumerate}
\item \textbf{\Biaseddataset{} - Certainty} The lower excepted utility \textit{Target} option is certain, while the other option with a higher excepted utility is given at some probability (\textit{Higher Excepted Value}).
\item \textbf{Control - No Certainty} The lower excepted utility \textit{Target} option has a higher probability, while the other option (\textit{Higher Excepted Value})  has a higher excepted utility with a lower probability.
\end{enumerate}

In both conditions, the probability gap between the options was held constant.
For instance, in the \biaseddataset{} condition, if one option was certain (100\%) and the other option had an 80\% chance of yielding a reward, the corresponding options in the control condition would have a 20\% probability gap.
% We obtained the values for prize rewards and probabilities from \cite{Kahneman1979ProspectTA} and also included additional values that maintained the same relationships.
% \nir{i would start the paragraph with this; otherwise readers will think we've invented this experimental paradigm (and only then find out we didn't)}

Similar to the decoy effect, we used a diverse set of prompts using 4 different sub-template combinations and options permutations to create our test set.

\begin{table*}[th!]
\centering
% \small
\begin{tabular}{@{}llccc  cc@{}}
\toprule
 &  & \multicolumn{3}{c}{\textbf{GPT3}} & \multicolumn{2}{c}{\textbf{T5}}  \\
 \cmidrule(lr){3-5} \cmidrule(lr){6-7}
& & \textbf{LM} &  \multicolumn{2}{c}{\textbf{Instruction-LM}} & \textbf{LM} & \textbf{Instruction-LM}  \\
\cmidrule(lr){4-5}
& \hspace{0.8cm} \textbf{Bias} & DaVinci & DaVinci-002 & DaVinci-003 & T5 & Flan--T5  \\
\midrule
\multirow{2}{*}{\rotatebox[origin=c]{90}{\textbf{}}} 
%& Certainty & 0.00 & 0.21* & \textbf{0.54}* & 0.09* & \textbf{0.16}*  \\ % this is 3 sub-types
%& Certainty & 0.00 & 0.24* & \textbf{0.67}* & 0.09* & \textbf{0.17}*  \\ % this is two main sub types
& Not Probable & 0.00 & 0.13* & \textbf{0.22}* & 0.08 & \textbf{0.14}*  \\ % this is not probable only
\bottomrule
\end{tabular}
\caption{The difference in bias scores between the choices of models in the target option in the \biaseddataset{} versus control conditions. A higher score means the model exhibits a higher level of bias. Results marked with * are statistically significant with p-values $<.05$.}
\label{tab:not_probable_results}
\end{table*}

\subsection{Belief Bias Data}

To explore the belief bias in LMs we conduct our experiments using the data generated by \citet{dasgupta2022language}.

% To explore the Belief bias in LMs we also conduct two experiments.
The model is presented with two premises and a conclusion and instructed to choose if the conclusion stems directly from the premises.
If the conclusion logically stems from the premises the model should output 'Valid', otherwise, it should output 'Invalid'.

Here there are two conditions, the bias condition where each argument is believable or unbelievable, and the control condition where the arguments are neutral in terms of believability.
% To control the effect of believability on the performance of the model we run a control experiment, in which we use a different set of objects in each experiment.
% \nir{not really clear what the treatment is at this point}

\begin{enumerate}
    \item \textbf{\Biaseddataset{} - Real-Life Objects } The objects the logical reasoning is based on \textit{real-life} objects, which can have believable or unbelievable nature according to world knowledge (e.g. ``cigarettes are addictive'' as believable, ``cigarettes are non-addictive'' as unbelievable).
    .\item \textbf{Control - Non-real Objects}  The objects the logical reasoning is based on our \textit{non-real} objects using made-up words, which do not have believable or unbelievable nature according to world knowledge (e.g ``wobars are shnesive'' and ``wobars are non-shnesive''), which create neutral arguments.
\end{enumerate}

The valid-believable and invalid-unbelievable conclusions in the condition of the Real-life object are considered as consistent conclusions and valid-unbelievable and invalid-believable are the inconsistent conclusions.
% In this bias, since there is a correct answer we can also measure the model accuracy on the task.
See \citet{dasgupta2022language} for more details on the belief bias data generation process.

% The real-life objects were taken from the original work on Belief bias \cite{evans1983conflict}.
% The non-real objects were created with made-up words that follow the grammatical English rules.

% To generate the non-real samples, we transformed each real-life sample by replacing each real-life object with a corresponding non-real object ("cigarettes" $\rightarrow$ "wobars"; "addictive" $ \rightarrow $ "shnesive").
% % This resulted in a set of non-real samples that were split into believable and unbelievable groups based on their alignment with real-life samples, even though believability has no meaning in the context of non-real objects.
% % This split allows for easier comparison of the results with those of real-life objects.

% We designed the data such that each conclusion could be either valid or invalid and believable or unbelievable, and we included an equal number of samples for each combination of attributes. To create a diverse set of samples, we used 5 different text templates and 3 different object sets, resulting in a total of 766 samples after permuting the premises.

% Beyond using our own data, we also used data from \cite{dasgupta2022language} where they used hand-crafted real-life objects which allow a higher level of unbelievability, and we report our result for both datasets.

\section{Not Probable Effect}
\label{appendix:sec:not_probable}

In the same work that presented the certainty effect, \citet{kahneman1979prospect} show another adjacent effect.
In this adjacent effect, people tend to underweight probabilities of outcomes that are possible but not probable (e.g. probabilities lower than 0.03), but overweight probabilities when they are merely probable.
% Section \ref{subsec:def_certainty} describe the certainty effect mentioned an additional bias associated with the certainty effect,
We name this adjacent effect \emph{not probable} effect, as demonstrated in the experiment conducted by \citet{kahneman1979prospect}.

In this experiment, participants were presented with choices between options that had the same expected utility value.
However, in the \biaseddataset{} condition, the probabilities associated with the options were exceptionally low, below 1\% winning chance, while in the control condition, the probabilities were substantial, above 10\% winning chance. Notably, the options offered the same prizes, and the ratio between the probabilities remained consistent.

According to the theory of expected utility, where both options have equal expected utility in both control and \biaseddataset{} conditions, the alteration in probabilities should not influence the choice.
Surprisingly, the results from \citet{kahneman1979prospect} indicated that when the probabilities were substantial (above 10\%), participants preferred the option with the higher probability and smaller prize.
In contrast, in the \biaseddataset{} condition, they favored the option with the larger prize and smaller probability.

To explore this bias further, we conducted similar experiments to the certainty bias, focusing on values that aligned with this bias.
The experimental findings on the model are presented in Table \ref{tab:not_probable_results}.
Consistently with other biases, these results demonstrate lower bias scores compared to the certainty effect.

\section{Differences Between Models}
\label{appendix:sec:diff_between_models}
%\input{Sections/Tables/diff_of_diffs}
% As mentioned in Section \ref{subsec:bias_score}, we measure how significant the differences in bias scores between models are by fitting linear regression models to predict the choice of the target option with regard to the dataset condition (control or \biaseddataset{}) and the type of model, also known as The difference-in-differences method \cite{dimick2014methods}.
% The linear regression is demonstrated in Equation \ref{appendix:eqa:diff_of_diff}, where $y$ is a binary label of whatever the model chose the target option of that sample, $M$ is the type of model, $T$ is whatever this sample is from the \biaseddataset{}  or control dataset and $\beta_{0},\beta_{1}, \beta_{2},\beta_{3}$ are the regression coefficients and $\epsilon$ allows for random noise.

To evaluate the significance of bias score differences between models (as explained in Section \ref{subsec:bias_score}), we utilize linear regression models based on the difference-in-differences method \cite{dimick2014methods}.
By considering the predictions of two models on both the control and \biaseddataset{} datasets, we train a linear regression model to predict the selection of the target option for each sample.
The regression model is provided with only two inputs: the model's identity and the dataset source for the given sample.

The linear regression is presented in Equation \ref{appendix:eqa:diff_of_diff}.
The binary label $y$ represents the target option choice, $M$ denotes the model type, $D$ indicates the dataset condition (control or \biaseddataset{}), and $\beta_{0}, \beta_{1}, \beta_{2}, \beta_{3}$ are the regression coefficients with $\epsilon$ accounting for random noise.

\begin{equation}
\label{appendix:eqa:diff_of_diff}
    y = \beta_{0} + \beta_{1} * M + \beta_{2} * D + \beta_{3} * M * D + \varepsilon
\end{equation}

The p-value of the interaction coefficient $\beta_{3}$ indicates the significance of differences in bias scores between models.    
By considering the bias score as the difference between datasets for the same model, the focus on the interaction coefficient enables us to directly quantify the extent of bias amplification across models influenced by the dataset condition.

% The p-value of the interaction coefficient $\beta_{3}$ between the dataset condition and the type of model state how much the differences in bias scores of different models are significant.

\paragraph{Results.}
As the vast majority of the differences are significant, we mention only the model pairs whose differences were \emph{not} significant (p-value < $0.05$).
We compare pairs of models within two models ``families'' - DaVinci, DaVinci-002, DaVinci-003, and GPT4 in one family, while T5 and Flan-T5 are in the other family.

% For the DaVinci and DaVinci-002 models, the difference was not significant in the belief valid, and in 3 out 4 products in decoy cheaper and in all products in decoy expensive.
% For the DaVinci-002 and DaVinci-003 models, the difference was not significant in two out of four products both in decoy cheaper and in decoy expensive.
% For the DaVinci-003 and GPT4 models, the difference was not significant in two out of four products in decoy cheaper and in one product in decoy expensive.
% For the T5 and Flan-T5, the difference was not significant in the certainty effect. 

For the DaVinci and DaVinci-002 models, the difference was not significant in the belief valid, and in decoy expensive.
For the T5 and Flan-T5, the difference was not significant in the certainty effect. 
All other biases and model pairs' differences were significant.

\section{Location-Dependent Choices}
\label{appendix:sec:options_locations}

\begin{table*}[th!]
\centering
% \small
\begin{tabular}{@{}llcc|c  cc@{}}
\toprule
 &  & \multicolumn{2}{c}{\textbf{Control}} & \multicolumn{3}{c}{\textbf{\Biaseddataset}}  \\
\cmidrule(lr){3-7}
 \hspace{0.7cm} \textbf{Model} &  \hspace{0.7cm} \textbf{Bias} & Option 1 & Option 2 & Option 1 & Option 2 & Option 3  \\
\midrule
\multirow{3}{*}{ \hspace{0.5cm} DaVinci} 
& Decoy Expensive &                             0.0\% &                           \textbf{100.0\%} &             0.0\% &                        2.2\% &                       \textbf{97.8\%} \\
 &   Decoy Cheaper &                             0.0\% &                           \textbf{100.0\%} &              0.0\% &                        1.5\% &                      \textbf{ 98.5\%} \\
 &       Certainty &            \textbf{ 100.0\%} &                         0.0\% &                     \textbf{ 100.0\%} &                        0.0\% &                       --- \\
 % &    Belief Valid &          74.0\% &                        26.0\% &                       74.0\% &                       26.0\% &                        0.0\% \\
 % &  Belief Invalid &      74.0\% &                        26.0\% &                       74.0\% &                       26.0\% &                        0.0\% \\
\midrule

\multirow{3}{*}{ \hspace{0.1cm} DaVinci-002} 
 & Decoy Expensive &                            71.5\% &                            28.5\% &          45.0\% &                       33.0\% &                       22.2\% \\
 &   Decoy Cheaper &                            75.5\% &                            24.5\% &             36.5\% &                       33.2\% &                       30.2\% \\
 &       Certainty &                    \textbf{ 87.0\%} &                        13.0\% &                       64.0\% &                       36.0\% &                       --- \\
 % &    Belief Valid &                     60.0\% &                        40.0\% &                       45.0\% &                       55.0\% &                        0.0\% \\
 % &  Belief Invalid &                      60.0\% &                        40.0\% &                       45.0\% &                       55.0\% &                        0.0\% \\
\midrule

\multirow{3}{*}{ \hspace{0.1cm} DaVinci-003} 
 & Decoy Expensive &                            77.0\% &                            23.0\% &      48.5\% &                       32.5\% &                       18.8\% \\
 &   Decoy Cheaper &                            79.0\% &                            21.0\% &      50.3\% &                       26.8\% &                       23.0\% \\
 &       Certainty &          57.0\% &                        43.0\% &                       44.0\% &                       56.0\% &                       --- \\
 % &    Belief Valid &      43.0\% &                        57.0\% &                       35.0\% &                       65.0\% &                        0.0\% \\
 % &  Belief Invalid &              43.0\% &                        57.0\% &                       35.0\% &                       65.0\% &                        0.0\% \\

\midrule

\multirow{3}{*}{ \hspace{0.7cm} GPT4} 
 & Decoy Expensive &                            63.0\% &                            37.0\% &           38.2\% &                       27.5\% &                       33.5\% \\
  &   Decoy Cheaper &                            78.0\% &                            22.0\% &          44.2\% &                       23.0\% &                       32.8\% \\
  &       Certainty &                    52.0\% &                        48.0\% &                       47.0\% &                       53.0\% &                        --- \\
  % &    Belief Valid &                     34.0\% &                        62.0\% &                       35.0\% &                       65.0\% &                        0.0\% \\
  % &  Belief Invalid &                     34.0\% &                        62.0\% &                       35.0\% &                       65.0\% &                        0.0\% \\
\midrule

\multirow{3}{*}{ \hspace{0.5cm} T5-XXL} 
 & Decoy Expensive &                            12.8\% &                            \textbf{87.2\%} &       33.5\% &                       47.0\% &                       20.0\% \\
 &   Decoy Cheaper &                            12.8\% &                           \textbf{ 87.2\%} &            33.2\% &                       48.8\% &                       18.0\% \\
 &       Certainty &                    31.0\% &                        69.0\% &                       32.0\% &                       68.0\% &                       --- \\
% &    Belief Valid &                      7.0\% &                        \textbf{93.0\% }&                        5.0\% &                       \textbf{95.0\%} &                        0.0\% \\
%  &  Belief Invalid &                       7.0\% &                        \textbf{93.0\%} &                        5.0\% &                      \textbf{ 95.0\%} &                        0.0\% \\

\midrule

\multirow{3}{*}{ \hspace{0.1cm} Flan-T5-XXL} 
 & Decoy Expensive &                            49.2\% &                            50.8\% &        45.2\% &                       35.0\% &                       20.0\% \\
 &   Decoy Cheaper &                            49.5\% &                            50.5\% &         44.0\% &                       25.8\% &                       30.0\% \\
 &       Certainty &                   44.0\% &                        56.0\% &                       38.0\% &                       62.0\% &                       --- \\
 % &    Belief Valid &                    32.0\% &                        68.0\% &                       28.0\% &                       65.0\% &                        0.0\% \\
 % &  Belief Invalid &               32.0\% &                        68.0\% &                       28.0\% &                       65.0\% &                        0.0\% \\
\bottomrule

\bottomrule
\end{tabular}
\caption{ Percentage of option location preferences across all samples for each model and bias.
The results reveal consistent patterns in the choice behavior of pretrained models, where DaVinci exhibits an absolute preference for a specific location in 100\% of the cases in the decoy and certainty effects. Similarly, T5-XXL shows a preference in over 87\% of the cases in the control decoy effects. In contrast, the remaining models exhibit varying tendencies towards specific option locations that are contingent upon the content of the options. Notably, DaVinci-002 demonstrates an 87\% preference for option 1 in the certainty effect.}
\label{tab:options_locations}
\end{table*}
To investigate the influence of option location on model preferences, we conducted experiments by permuting the order of options.
This approach allowed us to assess whether a model's preference for a particular option was driven by its location rather than its content.

While this permutation technique effectively controlled for the potential confounding effect of option location, it also provided insights into the prevalence of location-dependent choice in each model.
Table \ref{tab:options_locations} presents the preference of each model for specific locations in each experimental condition.

The table demonstrates that the pretrained models exhibit a strong reliance in most cases on option location in their decision-making process.
This reliance could explain their seemingly arbitrary choices and especially DaVinci's low bias scores, which are close to approximately -- 0.17 in the decoy effects and 0 in the certainty effect.

% This influence of option location could be affected by the DC-PMI correction we apply on the pretrained models as described in Section \ref{subsec:eval_ans}, as a high probability for a baseline prompt (e.g. "Answer: Option 2") could tilt the normalized model answers which we report to favor other options (since each answer is normalized by its baseline prompt probability.)
% We, therefore, verify in a partial experiment for the DaVinci model that shows that for the decoy and certainty effects they indeed prefer option by location even without the DC-PMI correction.

\section{GPT4 is Undecided}
\label{appendix:gpt4_zero-shot}
The results for the zero-shot for all biases can be viewed in Table \ref{appendix:gpt4_zero-shot}.
These results show similar trends to the 1-shot GPT4 results in Table \ref{tab:gpt4_results}, although the biases score are higher as a result of the few-shot improvement discussed in Section \ref{subsec:few_shot}.

When testing GPT4 on the certainty effect in the zero-shot settings, we noticed that in a large number of cases (about 17\%), the model does not choose one of the options. 
Instead, GPT4 responded with statements such as ``It's impossible to tell'' or ``As an AI, I don't have personal preferences'' and in some cases, the model explained that it needs to calculate the higher expected utility values step-by-step, and proceed by doing the calculation, completely avoiding the possibility for a bias.

In the few-shot setting, the model successfully adapted itself and provided a clear answer in the appropriate format.
For the bias scores presented in Table \ref{appendix:gpt4_zero-shot} we only considered examples where the model provided a clear answer.

\begin{table}[th]
\centering
\begin{tabular}{@{}lc|cc}
\toprule
 & \multirow{2}{*}{\textbf{Bias}}  & \multicolumn{2}{c}{\textbf{Zero-Shot}} \\
& & \textbf{DaVinci-003} & \textbf{GPT4} \\
\midrule
\multirow{5}{*}{\rotatebox[origin=c]{90}{\textbf{Bias Score}}} 
& Decoy Expensive &  -- 0.14 & \textbf{0.42}*   \\
& Decoy Cheaper &  0.16 & \textbf{0.20}*   \\
%& Certainty & \textbf{0.54}* & 0.17*   \\ % all three bias types
& Certainty & \textbf{0.67}* & 0.23*   \\ % two bias types
& Belief Valid & \textbf{0.23}* & 0.07*   \\
& Belief Invalid &  \textbf{0.61}* & 0.49*  \\
\bottomrule
\end{tabular}
\caption{comparison of the results between GPT4 and the most recent GPT3.5 release DaVinci-003 in zero-shot setting and zero-shot format. The decoy results are only on one product type (real-estate properties). Scores marked with * are statistically significant with p-values $<.05$}
\label{tab:gpt4_zero-shot_results}
\end{table}

% 0 and 1 shot at once!
%
% \begin{table*}[th]
% \centering
% \begin{tabular}{@{}lccc|cc}
% \toprule
%  & \multirow{2}{*}{\textbf{Bias}} & \multicolumn{2}{c}{\textbf{0-Shot}} & \multicolumn{2}{c}{\textbf{1-Shot}} \\
% & & \textbf{Text-DaVinci-003} & \textbf{GPT4} & \textbf{Text-DaVinci-003} & \textbf{GPT4} \\
% \midrule
% \multirow{4}{*}{\rotatebox[origin=c]{90}{\textbf{Bias Score}}} 
% & Decoy Expensive &  -- 0.14 & \textbf{0.42}* & NA & 0.38*  \\
% & Decoy Cheaper &  0.16 & \textbf{0.20}*  & NA  & 0.05  \\
% & Certainty & \textbf{0.54}* & 0.17*  & 0.35  & 0.15*  \\
% & Belief Valid & \textbf{0.23}* & 0.07*  & 0.21 & 0.06*  \\
% & Belief Invalid &  \textbf{0.61}* & 0.49*  & 0.51  & 0.28*  \\
% \bottomrule
% \end{tabular}
% \caption{comparison of the results between GPT4 and the most recent GPT3.5 release 'Text-DaVinci-003' in zero-shot setting and 1-shot format. Scores marked with * are statistically significant with p-values $<.05$}
% \label{tab:gpt4_results}
% \end{table*}

\section{Few-shots For Pretrained LM}
\label{appendix:sec:few_shot_pretrained}
\begin{figure}[t!]
\centering
\begin{subfigure}[t]{0.5\textwidth}
\centering
    \includegraphics[width=1\linewidth]{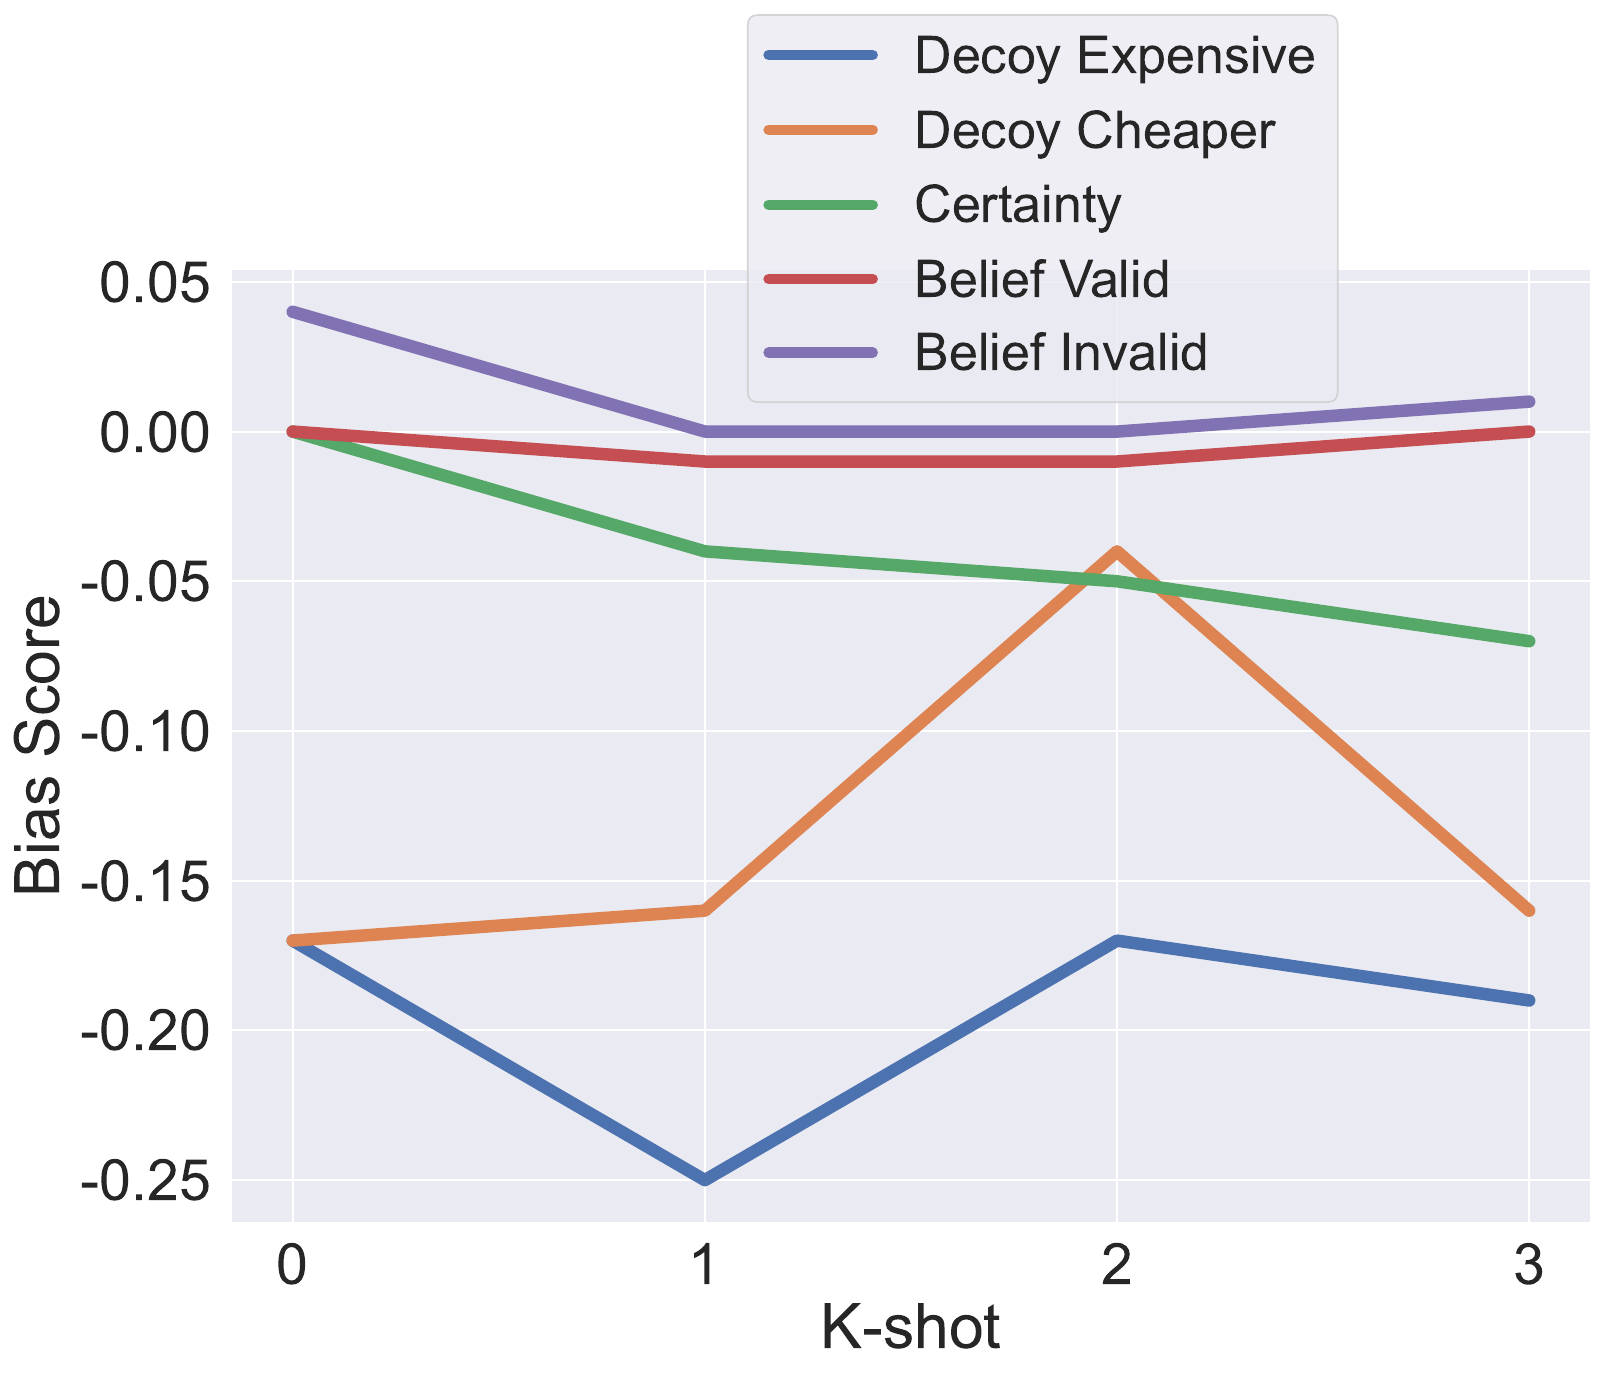}
    \caption{DaVinci}
    \label{fig:few_shot_davinci}
\end{subfigure}%
\hfill
\begin{subfigure}[t]{0.5\textwidth}
\centering
    \includegraphics[width=1\linewidth]{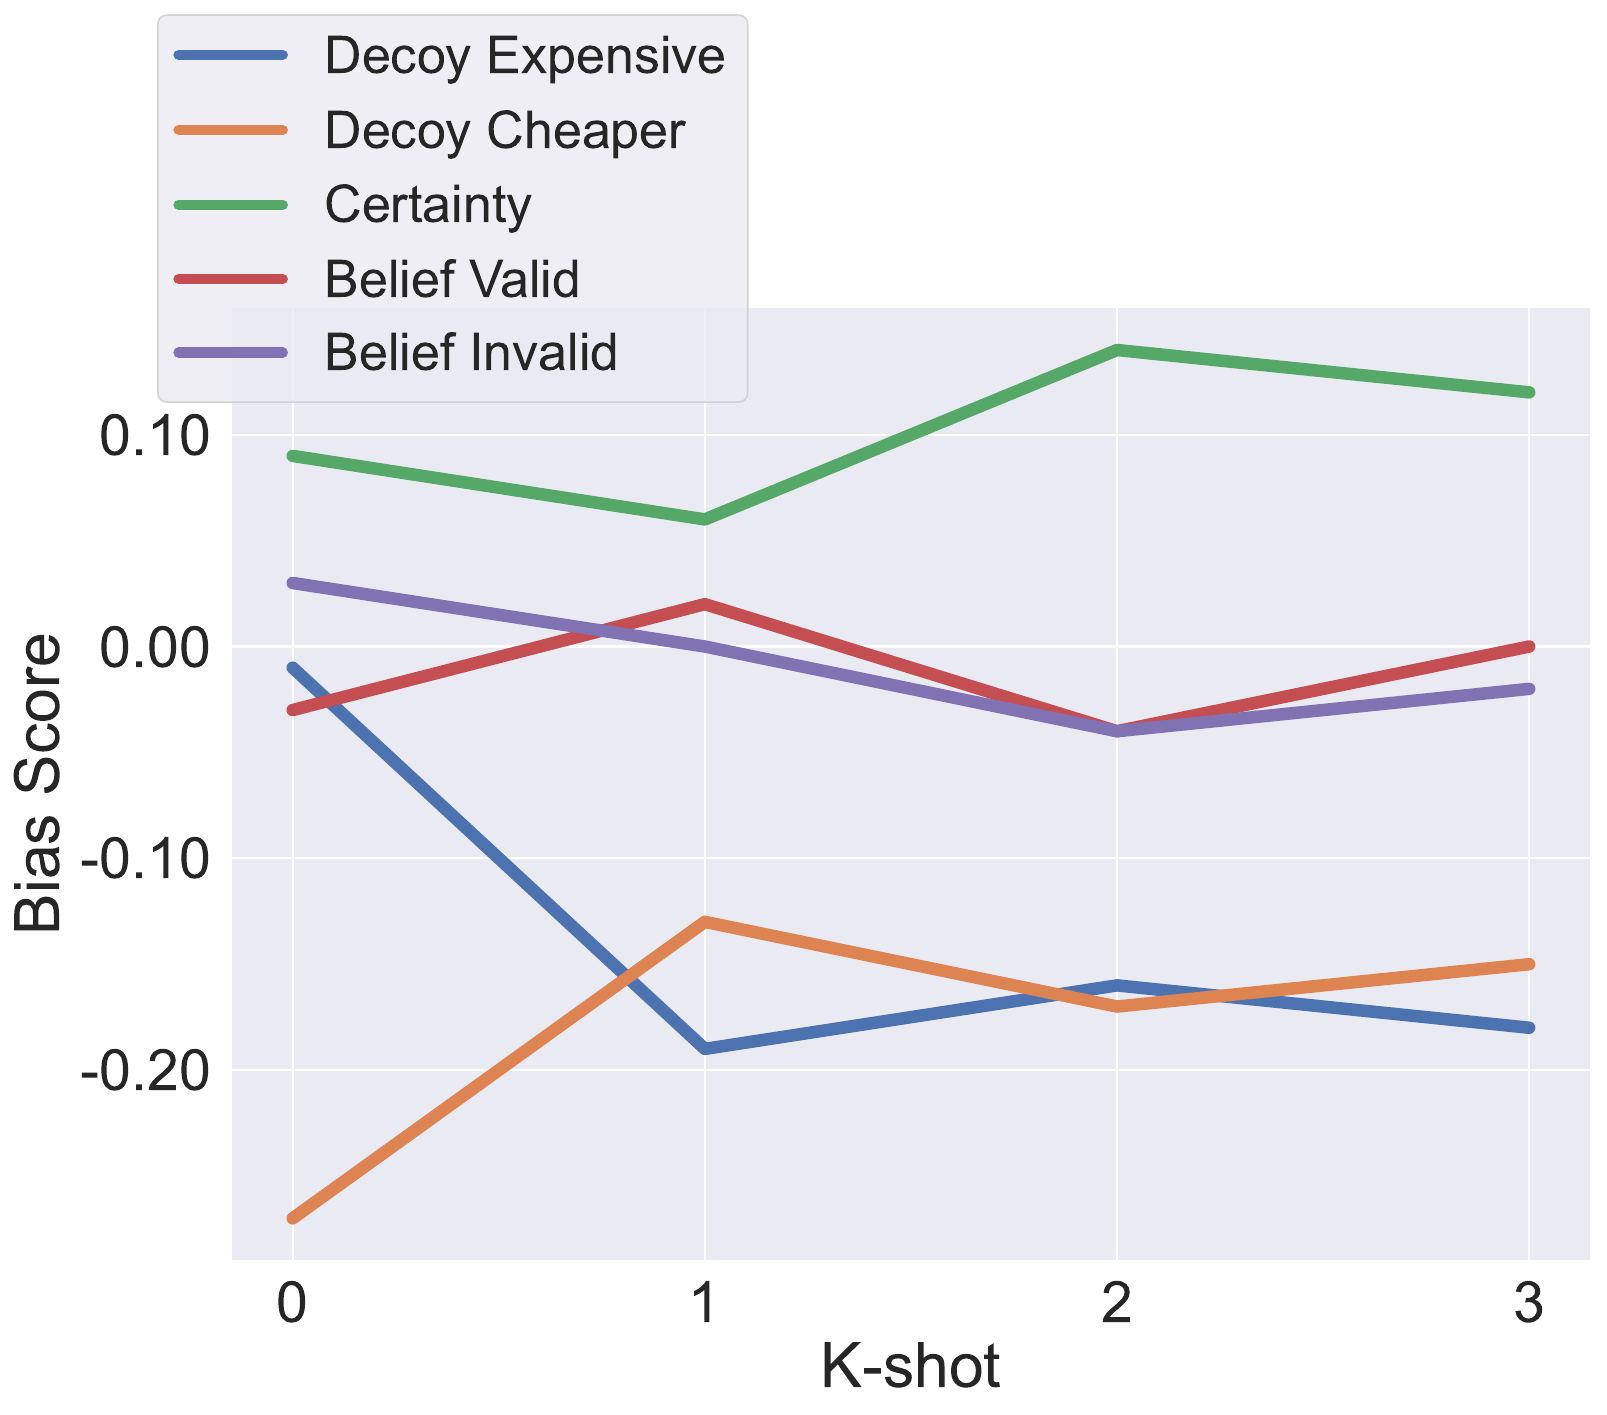}
    \caption{T5-XXL}
    \label{fig:few_shot_T5}
\end{subfigure}
\caption{The impact of format few-shots on bias scores in pretrained LLMs. The utilization of few-shot examples does not results in a significant change in bias scores.}
\label{fig:few_shot_pretrained}
\end{figure}
We can see the results for the pretrained models in Figure \ref{fig:few_shot_pretrained}.
As can be seen, using few-shot examples for the pretrained LM does not change the bias scores in a significant way.
That is in contrast to the minor drop in bias scores for their counterparts' instruction-tuned models, thus suggesting that the reason the pretrained models show smaller bias scores than the instruction-tuned models is not the fact that they fail to compile to the format of choice.

\begin{figure}[th!]
\centering
\includegraphics[width=1\columnwidth]{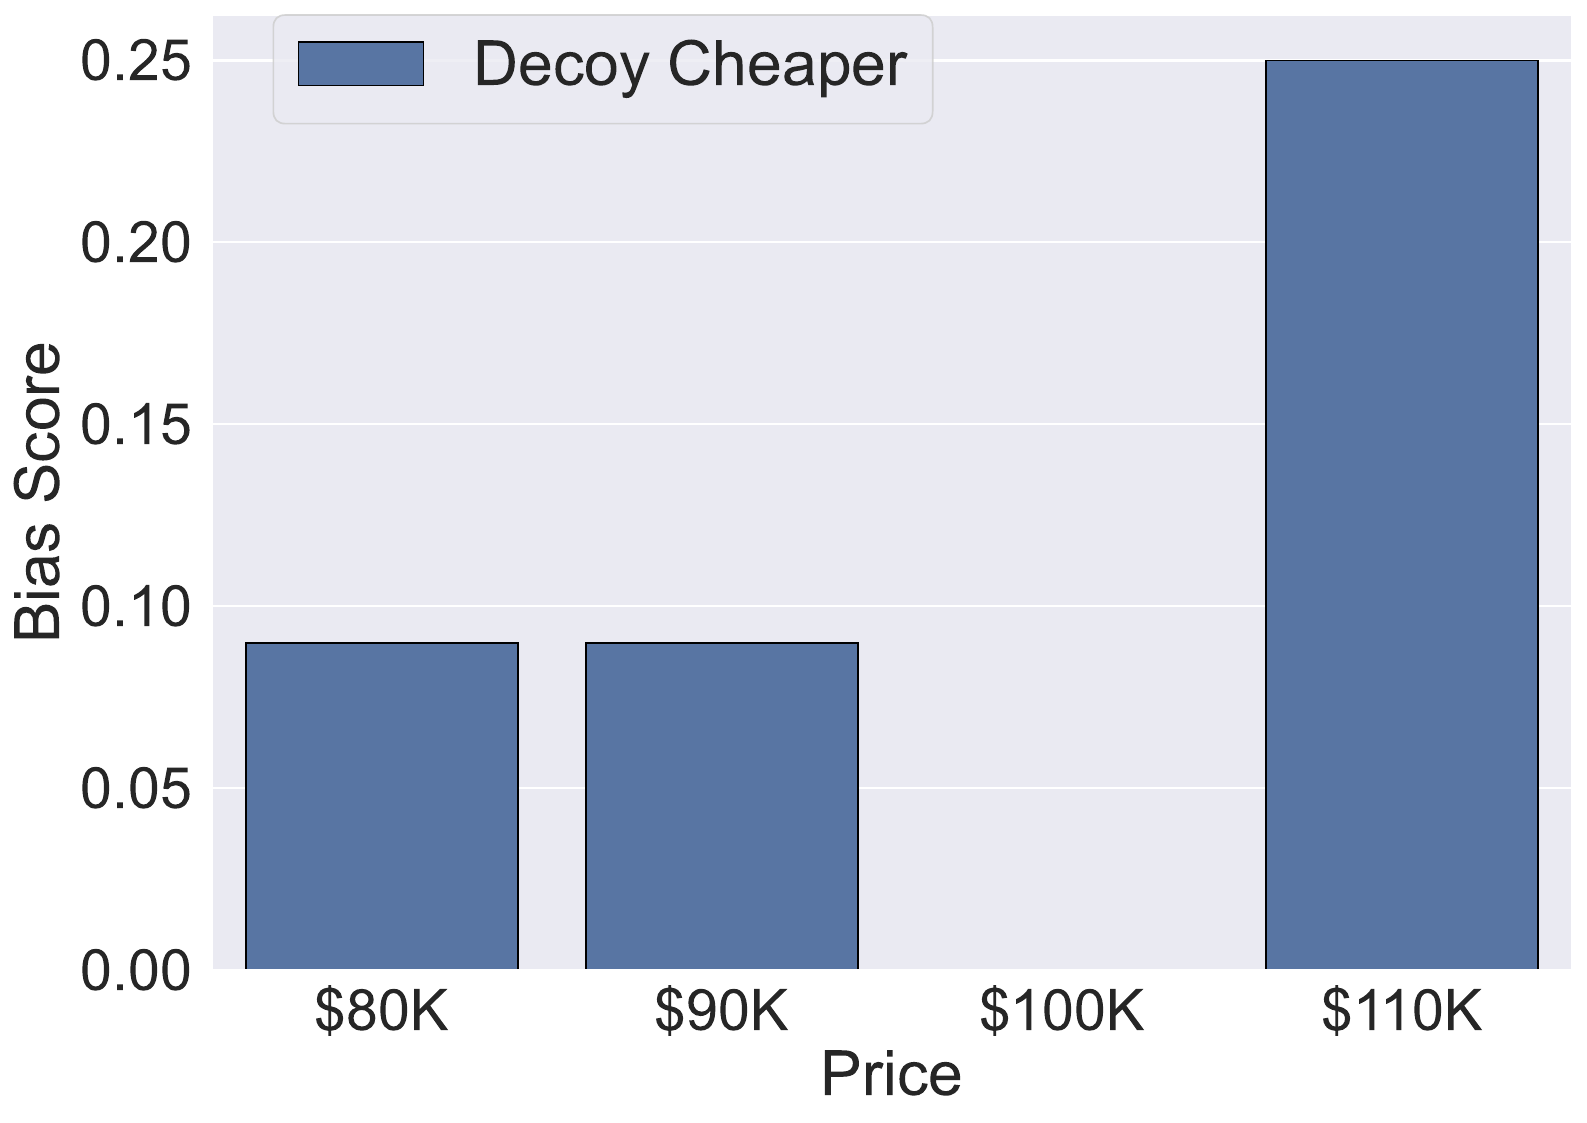}
% \qquad\qquad
\caption{The Effect of price range on the bias score of the decoy cheaper bias with real-estate products in the Flan-T5-XXL model. The x-axis represents the target price, where an increase in the target price leads to a wider gap between the target and competitor prices. The bias score demonstrates a positive correlation with the increasing price gap, except for the \$100K price where the model chose the competitor 100\% of the time.}
\label{fig:decoy_prices_flan}
\end{figure}

\section{Additional Analysis}
\label{appendix:sec:additional_analysis}

We add additional analysis results regarding the decoy effect in Sections \ref{appendix:subsec:price_range} and \ref{appendix:subsec:decoy_type_davinci003}, certainty effect in Section \ref{appendix:subsec:certainty_analysis} and the belief bias in Section \ref{appendix:subsec:belief_acc_bias_t5}.

\begin{table*}[th!]
\centering
% \small
\begin{tabular}{@{}llccc  cc@{}}
\toprule
 &  & \multicolumn{3}{c}{\textbf{GPT3}} & \multicolumn{2}{c}{\textbf{T5}}  \\
 \cmidrule(lr){3-5} \cmidrule(lr){6-7}
& & \textbf{LM} &  \multicolumn{2}{c}{\textbf{Instruction-LM}} & \textbf{LM} & \textbf{Instruction-LM}  \\
\cmidrule(lr){4-5}
\hspace{1.2cm} \textbf{Bias} & \hspace{0.3cm} \textbf{Product} & DaVinci & DaVinci-002 & DaVinci-003 & T5 & Flan--T5  \\
\midrule

\multirow{4}{*}{{\hspace{0.3cm} \textbf{Decoy Expensive}}} 
& Frying Pan & -- 0.12*  &  \hspace{0.1cm}  -- 0.23* & \textbf{-- 0.06} &  \hspace{0.15cm} \textbf{0.14}* &  -- 0.19*  \\
& Phone & -- 0.16* & -- 0.08 &  \hspace{0.1cm} \textbf{0.03} &  \hspace{0.15cm} \textbf{0.10}* & -- 0.09*   \\
& Car & -- 0.16* & -- 0.07  & \hspace{0.2cm} \textbf{0.09}* & -- \textbf{0.15}* &  -- 0.24*  \\
& Real-Estate & -- 0.17* & -- \textbf{0.13}*  &  \hspace{0.05cm} -- 0.14* & -- \textbf{0.01}  &  -- 0.19*  \\

\midrule

\multirow{4}{*}{{\hspace{0.2cm} \textbf{Decoy Cheaper}}} 
& Frying Pan & -- 0.18* &  \hspace{0.1cm} 0.03 &  \hspace{0.1cm} \textbf{0.11}* &  \hspace{0.1cm} -- 0.06 &  \textbf{0.22}*  \\
& Phone & -- 0.17* & -- 0.10* & \textbf{0.01}  & -- 0.10* &  \textbf{0.35}*  \\
& Car & -- 0.17* & -- 0.12*  & \textbf{0.04}  & -- 0.15*  &  \textbf{0.16}*  \\
& Real-Estate & -- 0.17* & -- 0.14* &  \hspace{0.1cm} \textbf{0.16}* &  -- 0.27* & \textbf{0.08}*   \\

\bottomrule
\end{tabular}
\caption{The bias scores for different products in the decoy expensive and decoy cheaper effects. A higher score means the model exhibits a higher level of bias. Results marked with * are statistically significant with p-values $<.05$.}
\label{appendix:tab:products_results}
\end{table*}
\subsection{Product Results}
\label{appendix:subsec:products_results}
The comprehensive product results for the decoy expensive and decoy cheaper effects are presented in Table \ref{appendix:tab:products_results}.
Similarly to the main results, we observe that the instruction-tuned models generally do not exhibit positive bias scores in the decoy expensive effect for most products.
Conversely, the decoy cheaper effect consistently yields higher positive bias scores across all products.

\subsection{Decoy Price Range}
\label{appendix:subsec:price_range}

Section \ref{subsec:decoy_analysis} presents the results concerning the influence of price range on the DaVinci-003 model decoy cheaper bias score.
Similarly, an analogous analysis was conducted on the Flan-T5-XXL model, and the outcomes are illustrated in Figure \ref{fig:decoy_prices_flan}.

The results demonstrate a similar trend to the DaVinci-003 model, with one exception: when the target price is \$100K, the bias score drops to 0.
Further investigation revealed that the Flan-T5-XXL model consistently favors the competitor in 100\% of the samples at this specific price point.

While the underlying reason for this behavior remains elusive, it is an intriguing finding that warrants future exploration. Understanding the fundamental preference patterns of the Flan-T5-XXL model, as well as other models in general, presents an avenue for future research.

\subsection{Decoy Sub-Type}
\label{appendix:subsec:decoy_type_davinci003}
\begin{figure}[th!] 
\centering
\includegraphics[width=1\columnwidth]{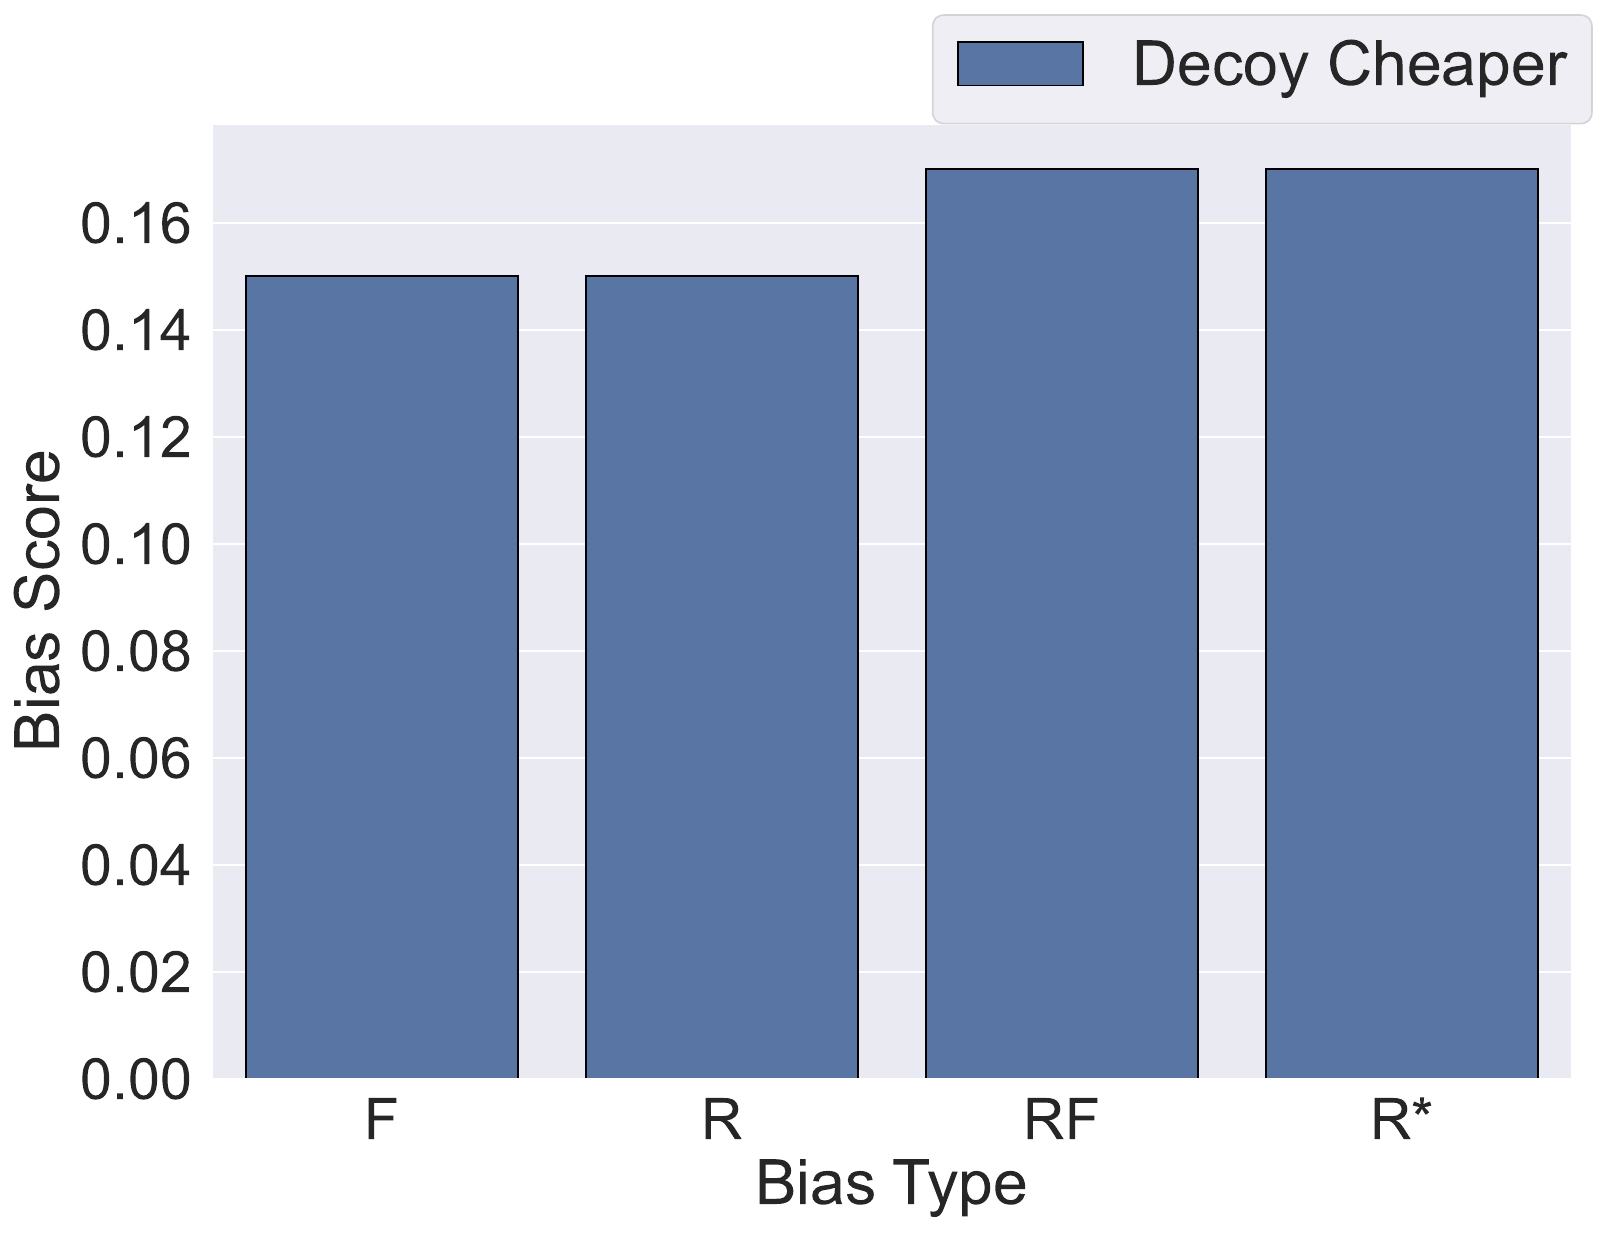}
\caption{The Impact of Decoy Sub-types on Decoy Cheaper Bias Score for Real-Estate Products in DaVinci-003. Sub-types include \textit{F} (same price, worse quality), \textit{R} and \textit{R*} (higher price, same quality), and \textit{RF} (higher price, worse quality). In contrast to humans, the DaVinci-003 model does not show a strong shift in bias score for different decoy sub-types.}
\label{fig:decoy_type_davinci003}
\end{figure}

In contrast to the notable effect observed in the Flan-T5 models with respect to the decoy sub-type, the DaVinci-003 model exhibits a consistent bias score across all sub-types, as depicted in Figure \ref{fig:decoy_type_davinci003}.

\subsection{Certainty Effect Analysis}
\label{appendix:subsec:certainty_analysis}
In a similar fashion to the price gap effect observed in the decoy effect, we can examine the impact of the target option's prize on the bias scores by varying the prize values presented to the model in the certainty effect options.

The results are illustrated in Figure \ref{fig:certainty_prize}.
While the Davinci-003 model exhibits a mostly consistent bias score across most prize values, the Flan-T5 model displays a sudden drop in bias scores for mid-range prizes, indicating lower biases in those cases.
The reason for this drop remains unclear and warrants further investigation.

Additionally, we conduct an analysis by categorizing the samples based on the utility gap between the two options.
The outcomes of this analysis are depicted in Figure \ref{fig:certainty_utility_gap}, showing a similar trend to the relationship between the prizes and bias scores and revealing that the bias score drop is probably not due to the utility gap.

These two analysis demonstrates that the bias is more stable in the DaVinci-003 model compared to the variation in the Flan-T5 model.
Future research could scale up the data and investigate more deeply the way different models are biased and how they are affected by the values of the different samples.

% \begin{figure}[t!]
% \centering
% \includegraphics[width=1\columnwidth]{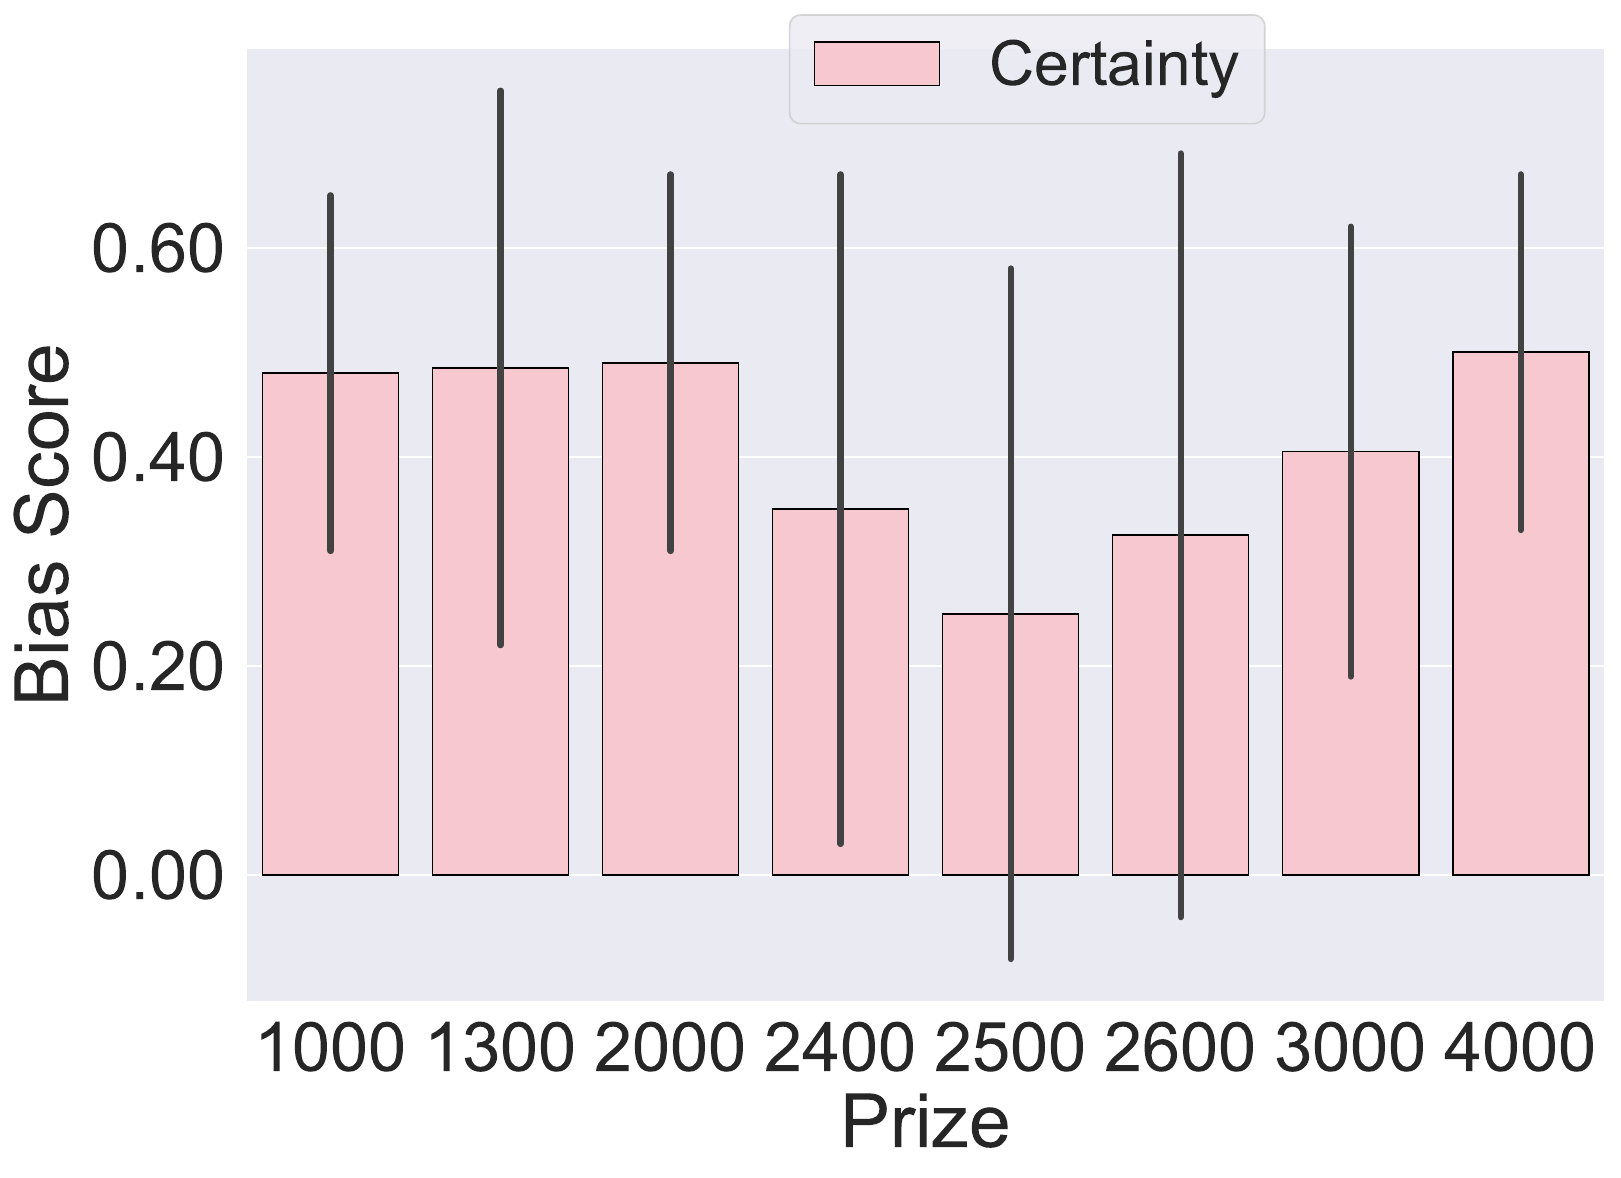}
% % \qquad\qquad
% \caption{The Effect of the Certainty different prize money in the target option on the bias score. X axis is the prize in dollars.}
% \label{fig:certainty_prize}
% \end{figure}
\begin{figure}[t!]
\centering
\begin{subfigure}[th!]{0.5\textwidth}
\centering
    \includegraphics[width=1\linewidth]{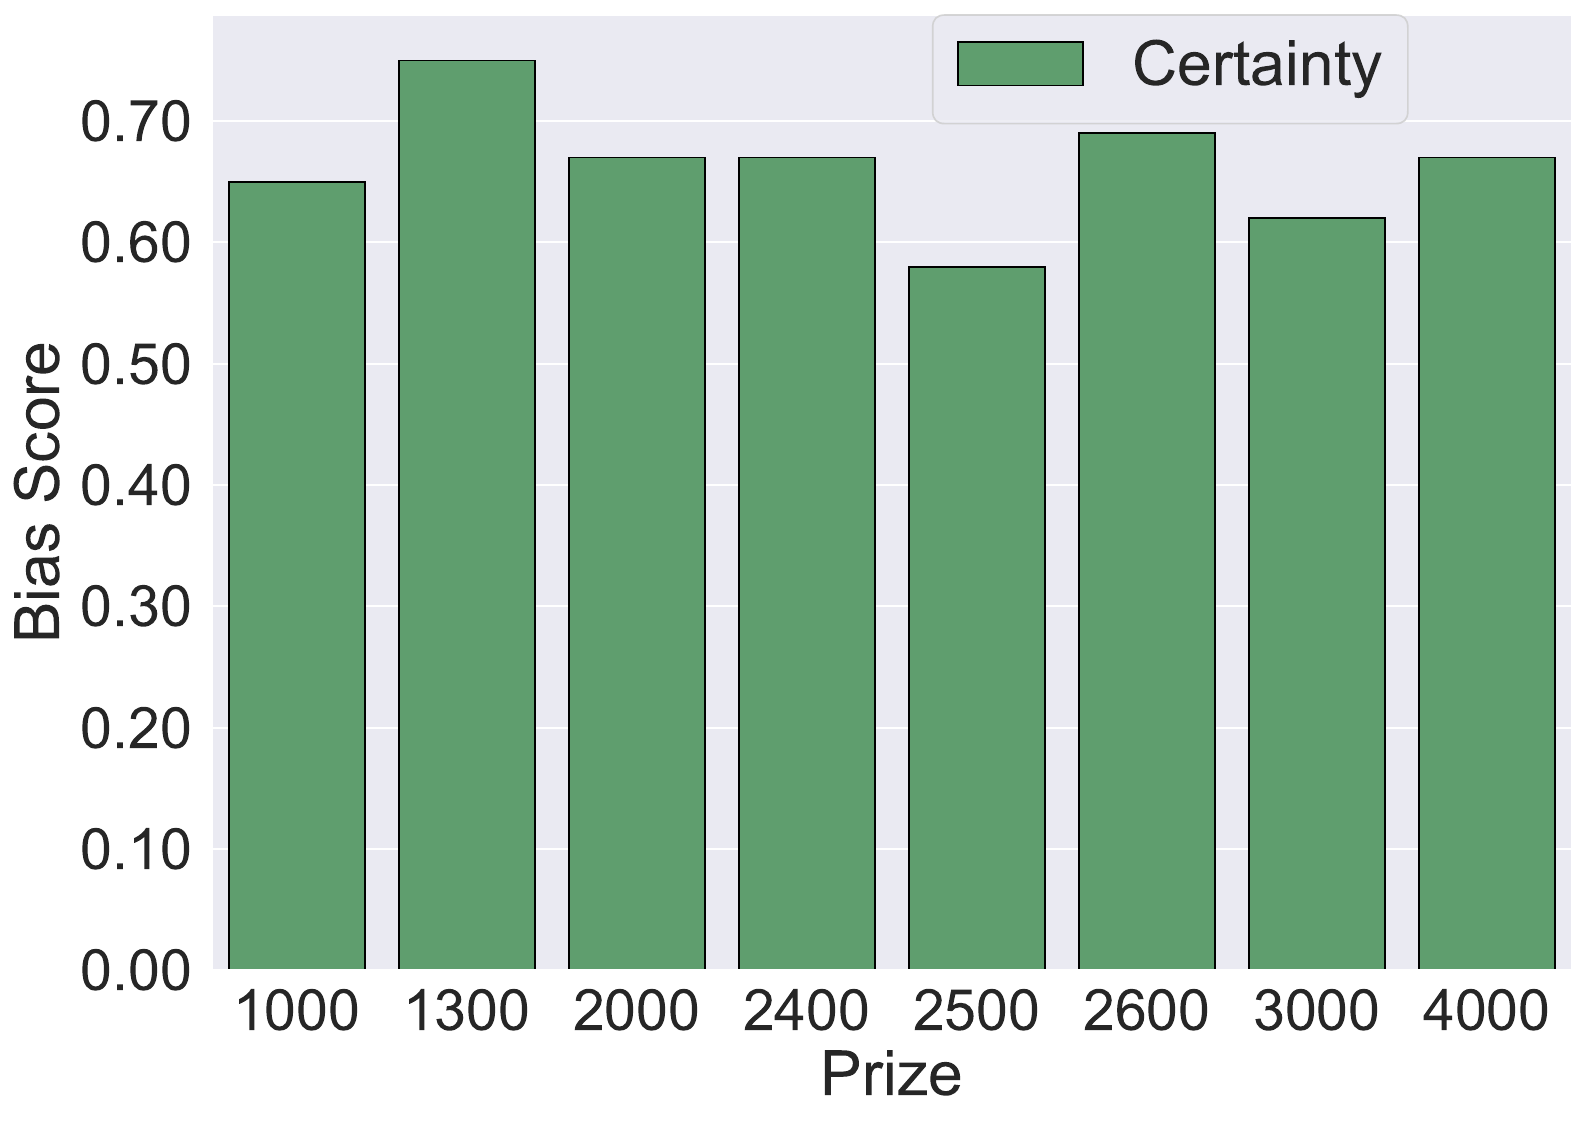}
    \caption{DaVinci-003}
    \label{fig:certainty_prize_davinci003}
\end{subfigure}%
\hfill
\begin{subfigure}[th!]{0.5\textwidth}
\centering
    \includegraphics[width=1\linewidth]{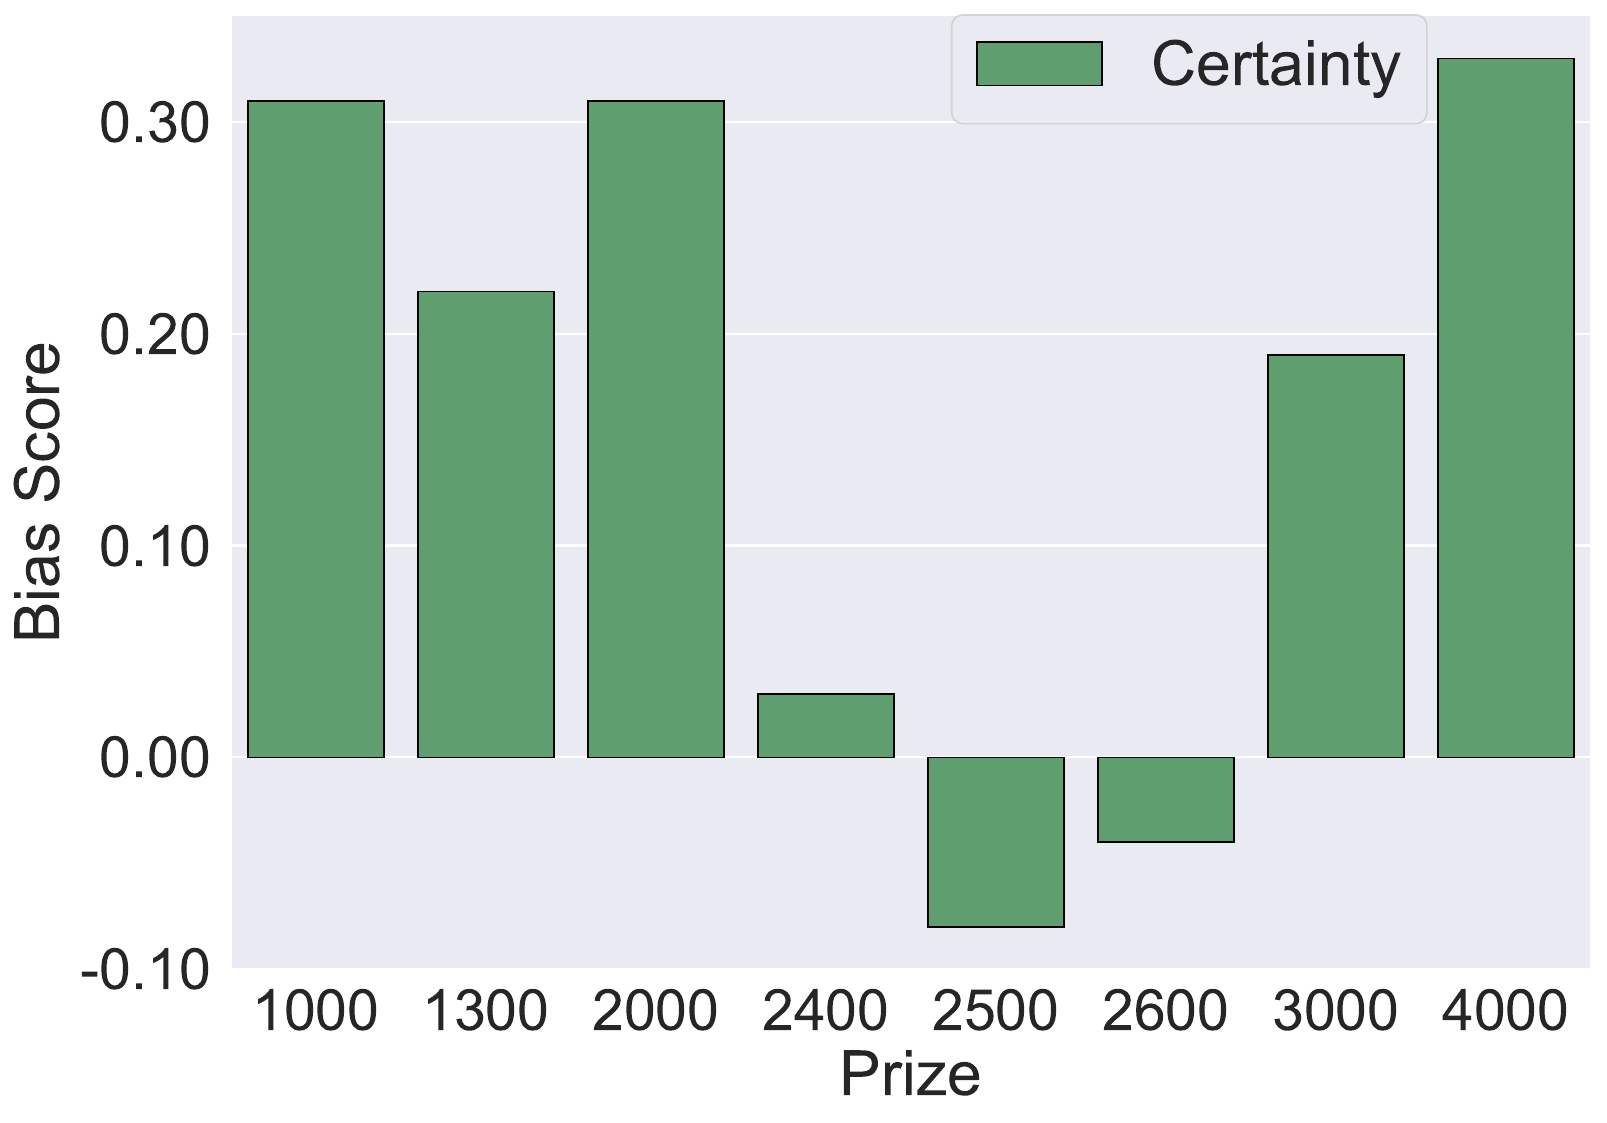}
    \caption{Flan-T5-XXL}
    \label{fig:certainty_prize_flan}
\end{subfigure}
\caption{The certainty effect bias scores impacted by different prize money in the target option. X axis is the prize in dollars.}
\label{fig:certainty_prize}
\end{figure}
\begin{figure}[t!]
\centering
\begin{subfigure}[th!]{0.5\textwidth}
\centering
    \includegraphics[width=1\linewidth]{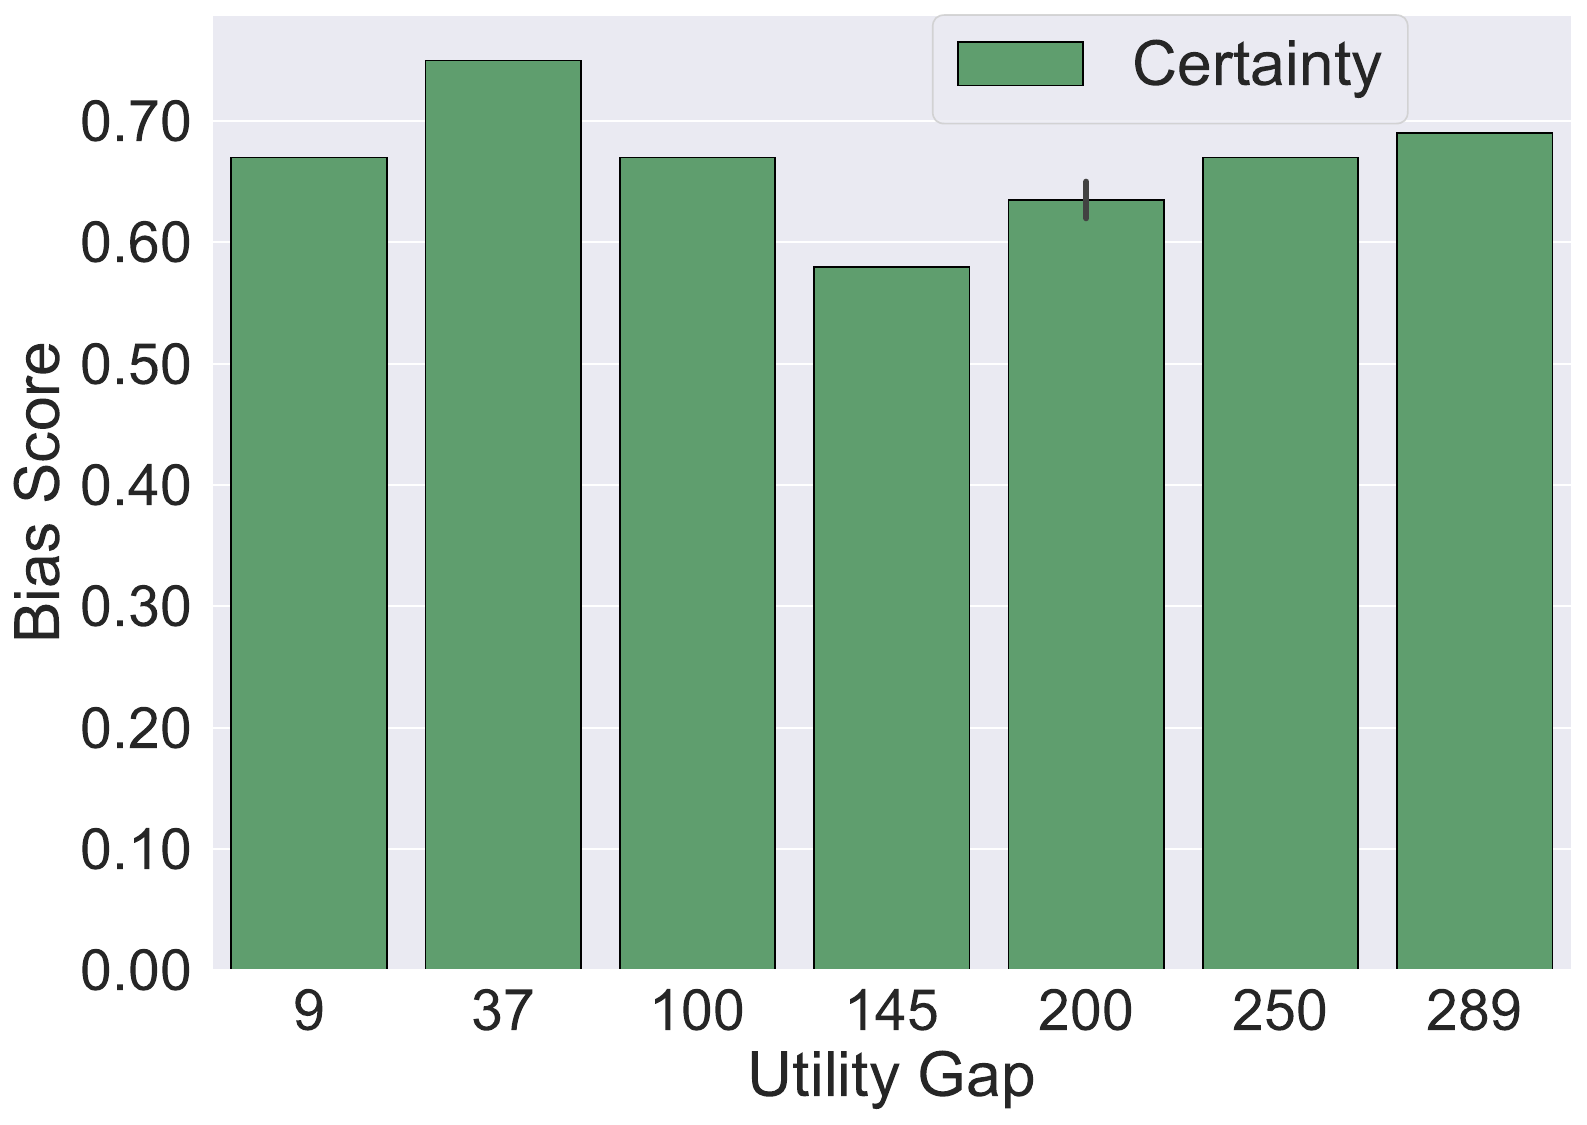}
    \caption{DaVinci-003}
    \label{fig:certainty_utility_davinci003}
\end{subfigure}%
\hfill
\begin{subfigure}[th!]{0.5\textwidth}
\centering
    \includegraphics[width=1\linewidth]{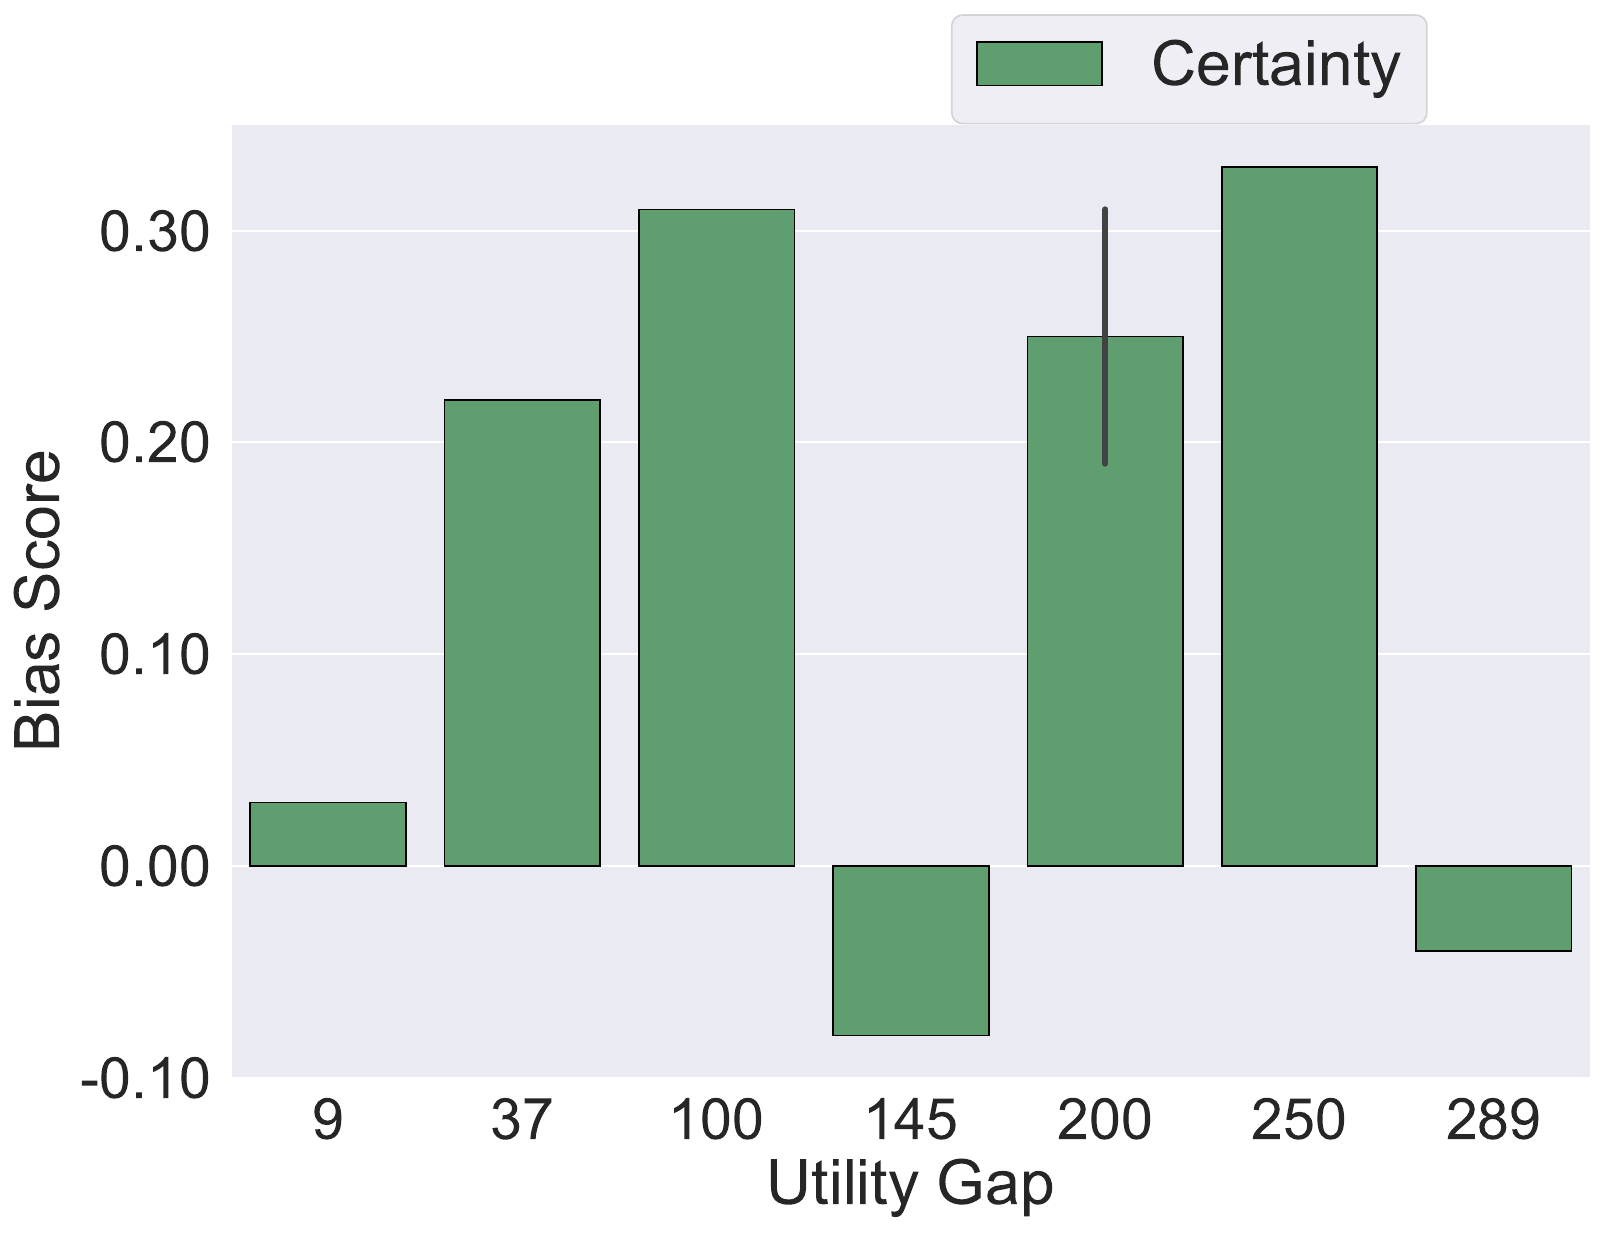}
    \caption{Flan-T5-XXL}
    \label{fig:certainty_utility_flan}
\end{subfigure}
\caption{The certainty effect bias scores are impacted by a utility gap between the higher expected value option to the target option. The x-axis is the utility gap.}
\label{fig:certainty_utility_gap}
\end{figure}

\subsection{Belief Bias}
\label{appendix:subsec:belief_acc_bias_t5}
\begin{figure}[t!] 
\centering
\includegraphics[width=1\columnwidth]{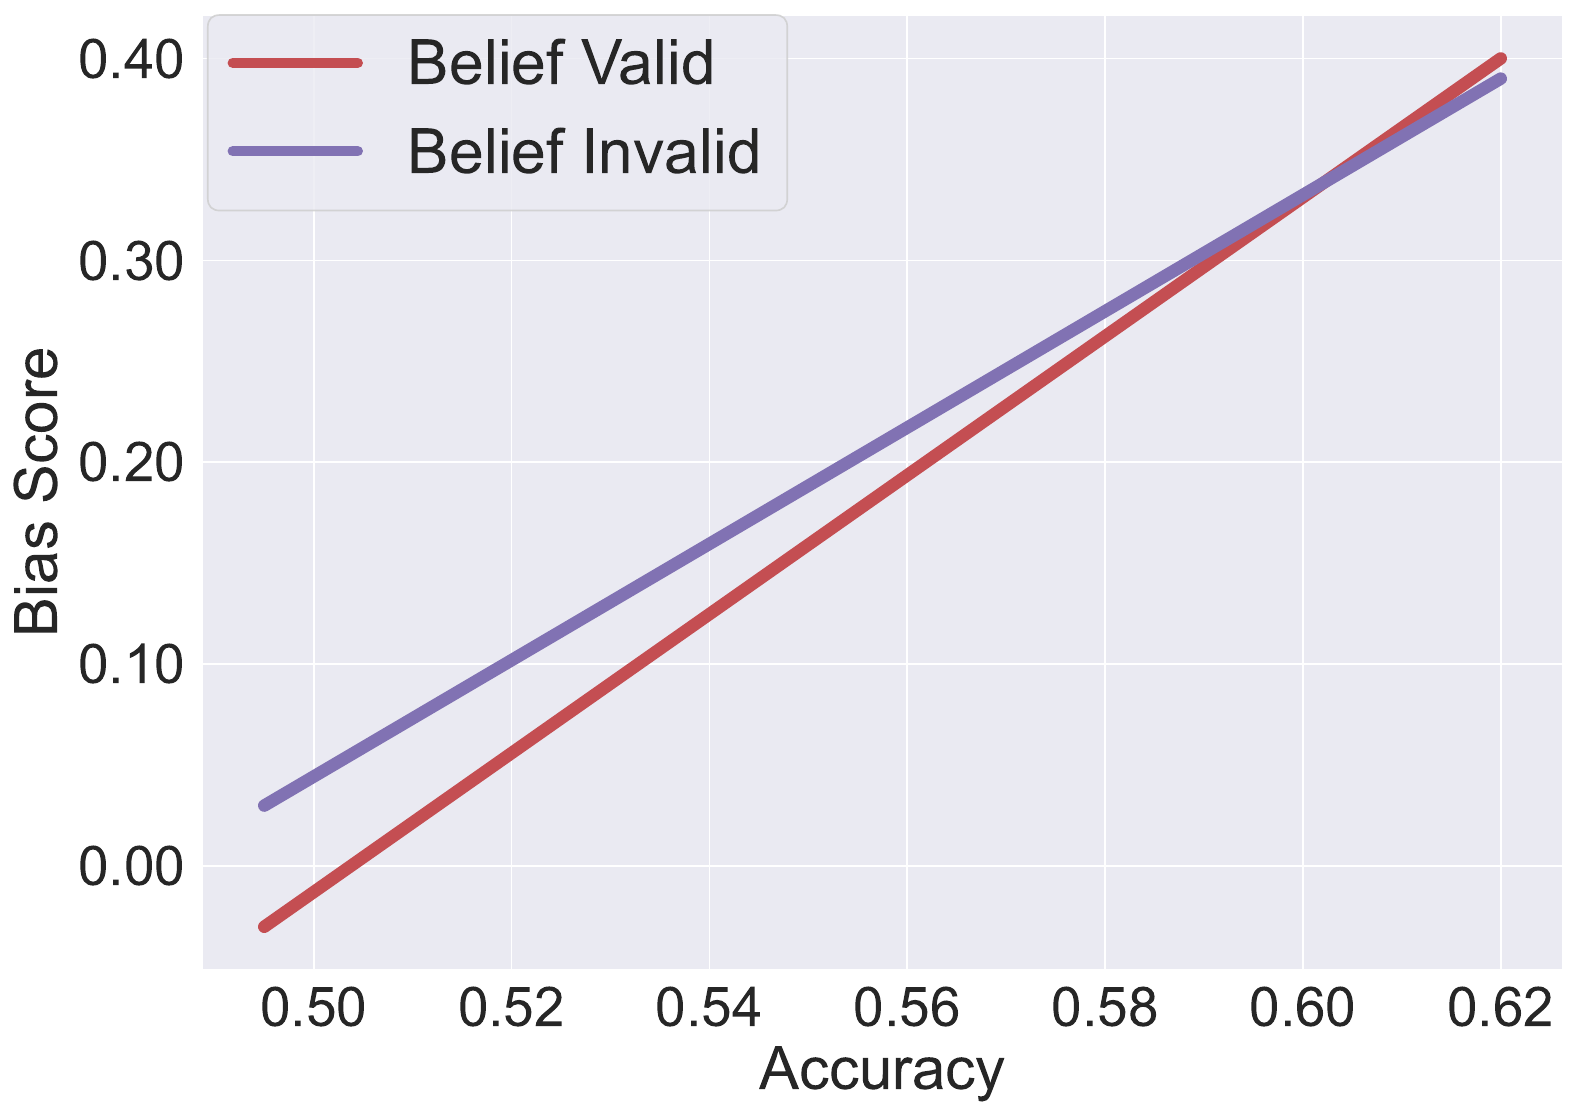}
% \qquad\qquad
\caption{The relationship between bias scores and model accuracy on the belief bias task's logical reasoning aspect for the T5-XXL and Flan-T5-XXL models. Similarly to the GPT models, an increase in model accuracy is accompanied by higher bias scores.}
\label{fig:belief_acc_bias_t5}
\end{figure}

Figure \ref{fig:belief_acc_bias_t5} showcases the change in bias scores relative to the accuracy of the T5 models on the logical reasoning aspect of the belief bias task with a similar trend to the GPT models.
